# Supplementary material for: Targeted Adversarial Training for Natural Language Understanding
Source: arXiv:2104.05847 source file (2021-04-12)
Supplement: Supplementary file 1 [file appendix.tex]

\section{Dataset Statistics}
\label{sec:data_stats}

The GLUE benchmark, SNLI, SciTail, HANS, MedNLI and XNLI datasets
are briefly introduced in the following sections. The
detailed description can be found in (\cite{wang2018glue}; \cite{scitail}; \cite{mccoy2019hans}; \cite{romanov2018mednli}; Khot et al., 2018; \cite{conneau2018xnli}) respectively. 



The statistics of all datasets used in this paper is summarized in \autoref{tab:datasets}.
The top four datasets in \autoref{tab:datasets} are used for training and the matched dev sets are used for both validation and in-domain evaluation.
The remaining datasets are used only for evaluation purpose. Among the evaluation datasets, other than BioASQ \cite{bioasq} from MRQA where the development set is used for evaluation, the corresponding test set is used for evaluating model out-of-domain generalization. 
